# Supplementary material for: Extending Model-x Framework to Missing Data
Source: arXiv:2202.13054 source file (2025-08-30)
Supplement: Supplementary file 1 [file appendix.tex]

% \section{Posterior Sampling, HMM}\label{post_hmm}

% \begin{algorithm}[H]

%     Input: $x_o, P_X$\\
%         \SetAlgoLined
%             $\hat{z}\sim P_{Z\mid X_o}(\cdot;x_o)$ \\
%             $\hat{x}_m \sim P_{X_m\mid Z}(\cdot;\hat{z}) $\\
%     Output: $\hat{x}_m$
% \end{algorithm}

% \input{tex/proof_lami}
% \input{tex/proof_mb}

\section{Algorithms}

\subsection{Univariate Sampled Imputation}
We describe how Theorem \ref{thm:uni} can be applied to N i.i.d. observations in Algorithm \ref{alg:uni}.

\begin{algorithm}[H]
\caption{Univariate sampled missing value knockoffs}\label{alg:uni}
\begin{algorithmic}
\STATE {\bfseries Input:} $\{x^{(i)}_{o^{i}}\}_{i=1}^N, \{m^{i},o^{i}\}_{i=1}^N, \{P_{\Xt_{o^i}\mid X_{o^i}}\}_{i=1}^N, P_X$
 \FOR{\texttt{$i=1,\dots,N$}}
    \STATE $m\leftarrow m^i$
    \STATE $o\leftarrow o^i$
    \STATE $\xt_o \sim P_{\Xt_o\mid X_o}(\cdot;x_o^{(i)}) $\hfill\COMMENT{Knockoff Sampling for $X_o$}
    \FOR {$j= 1,...,|m|$}
        \STATE $\hat{x}_{m_j}\sim P_{X_{m_j}}(\cdot)$\hfill\COMMENT{Uni. Imputation of Originals} 
        \STATE $\xt_{m_j}\sim P_{X_{m_j}}(\cdot)$\hfill\COMMENT{Uni. Imputation of Knockoffs} 
    \ENDFOR
    \STATE $\hat{x}^{(i)}\leftarrow(x_o^{(i)},\hat{x}_m)$
    \STATE $\xt^{(i)}\leftarrow(\xt_o,\xt_m)$
\ENDFOR
 \STATE {\bfseries Output:} $x_c,\xt$ 
\end{algorithmic}
\end{algorithm}

\subsection{HMM Latent Variable Posterior Sampling}

% \section{
Given $x_o$, we define $o(t)\defeq o\cap\{1,\dots,t\}$. Algorithm \ref{alg:hmm_post} is an extension of the ``Forward backward sampling for a HMM'' of \cite{sesiaGeneHuntingHidden2019} to the missing data setting. In the missing data setting, multiplication with the emission probabilities $P_{X_t\mid Z_t}$ needs to be applied only if $t$ is observed. That is equivalent to setting the emission probabilities to one for missing values as discussed in
\cite{broman2009guide} Appendix D.2. We provide the theoretical justification in Prop. \ref{thm:hmm_post} for completeness.

\begin{algorithm}[H]
\caption{HMM Latent Posterior Sampling with Missing Values}\label{alg:hmm_post}
\begin{algorithmic}
\STATE {\bfseries Input:} $x_o, P_{Z_1}, P_{X\mid Z}$,$P_{\Zt \mid Z}, o$
\FOR{\texttt{$t=1,\dots,T$}}
    \IF{ $t=1$}
        \STATE $\alpha_t(z_t) \leftarrow P_{Z_1}(z_1)$
    \ELSE 
        \STATE $\alpha_t(z_t) \leftarrow  \sum_{z_{t-1}}P_{Z_t\mid Z_{t-1}}(z_t; z_{t-1})\alpha_{t-1}(z_{t-1})$
    \ENDIF
    \IF{$t\in o$}
    \STATE $\alpha_t(z_t) \leftarrow \alpha_t(z_t)P_{X_t\mid Z_t}(x_t;z_t)$
    \ENDIF
\ENDFOR
\FOR{\texttt{$t=T,\dots,1$}}
    \IF{$t=T$}
        \STATE $P_{\hat{Z}_T\mid X_{o}}(z_T;x_{o})\leftarrow\dfrac{\alpha_{t}(z_t)}{\sum_{z_t'}\alpha_{t}(z_t')}$
        \STATE $\hat{z}_T\sim P_{\hat{Z}_T\mid X_{o}}(\cdot;x_{o})$
    \ELSE
        \STATE $P_{\hat{Z}_t\mid \hat{Z}_{t+1},X_{o(t)}}(z_t;z_{t+1},x_{o(t)})\leftarrow\dfrac{P_{Z_{t+1}\mid Z_t}(z_{t+1};z_t)\alpha_{t}(z_t)}{\sum_{z_t'}P_{Z_{t+1}\mid Z_t}(z_{t+1};z_t')\alpha_{t}(z_t')}$
        \STATE $\hat{z}_t\sim P_{\hat{Z}_t\mid \hat{Z}_{t+1},X_{o(t)}}(;\hat{z}_{t+1},x_{o(t)})$
    \ENDIF
\ENDFOR
\STATE {\bfseries Output:}  $\{\hat{z_t}\}_{t=1}^T$ 
\end{algorithmic}
\end{algorithm}
\section{Proofs}\label{app:proof}
\subsection{Theorem \ref{thm:uni}}\label{app:uni}

\textbf{Correction:} In the submitted manuscript, we have denoted that \pe of Theorem \ref{thm:uni} holds for both MAR and MCAR. We're weren't able to prove the statement under MAR and decided to restrict the theorem to the MCAR setting. The revised Theorem \ref{thm:uni} is given below:

\newtheorem*{thm*}{Theorem}

\begin{thm*}\label{thm:corrected}

Let $\Xh=(\Xh_1,\dots,\Xh_p)^T$ denote the imputed vector where $\Xh_o=X_o$ and ${\hat{X}_{m_j}\sim P_{X_{m_j}}(\cdot) \ j=1,\dots, |m|}$. We assume $P_{X,R}$ satisfies MCAR. If $\Xt_o \sim P_{\Xt_o\mid X_o}(\cdot;\hat{X_o})$, $P_{\Xt_o\mid X_o}$ is pairwise exchangeable with respect to $P_{X_o}$, and $\Xt_{m_j}\sim P_{X_{m_j}}(\cdot) \ j=1,\dots, |m|$ then $\hat{X}$ and $\Xt$ are pairwise exchangeable.
\end{thm*}

To prove Theorem \ref{thm:corrected} we first show a useful lemma regarding the \pety of fully factored joint distributions.

\begin{lem}\label{lem:factor}
If ${\displaystyle P_X(x)=\prod_{j=1}^{p} P_{X_j}(x_j)}$ and $P_{\Xt}(x)=P_X(x)$, then $X,\Xt$ are \pe.
\end{lem}
\begin{proof}
Following Prop. 3.5.  of \cite{candesPanningGoldModelX2017}, $X,\Xt$ are \pe iff for all index $j\in\{1,\dots,p\}$, 

\begin{equation}\label{eq:iff}
    P_{X_j,\Xt_j,X_{-j},\Xt_{-j}}(x_j,\xt_j,x_{-j},\xt_{-j})=P_{X_j,\Xt_j,X_{-j},\Xt_{-j}}(\xt_j,x_j,x_{-j},\xt_{-j})
\end{equation}

We now show when $P_X$ fully factors Eq. \ref{eq:iff} holds.
% \begin{subequations}\label{proof:uni}
% \begin{align}
\begin{equation}
    \begin{split}
        P_{X_j,\Xt_j,X_{-j},\Xt_{-j}}(x_j,\xt_j,x_{-j},\xt_{-j})&=P_{X_j}(x_j)P_{X_j}(\xt_j)\prod_{l\neq j}P_{X_l}(x_l)P_{X_l}(\xt_l)\\
        &=P_{X_j}(\xt_j)P_{X_j}(x_j)\prod_{l\neq j}P_{X_l}(x_l)P_{X_l}(\xt_l)\\
        &=P_{X_j,\Xt_j,X_{-j},\Xt_{-j}}(\xt_j,x_j,x_{-j},\xt_{-j})
        % &=P_{X_o,X_m}(x_o,\hat{x}_m)
\end{split}
\end{equation}

% \begineq
\end{proof}

\begin{proof}[Proof of Theorem \ref{thm:uni}]
% Let $x=(x_o,x_m)^T$,

For all missing data masks $ r\in \{0,1\}^{p}$, because the missing values are sampled from an univariate distribution, the distribution $P_{\Xh_m,\Xt_m\mid R}(\xh_m,\xt_m;r)$ fully factors out i.e.
\[
        P_{\Xh_m,\Xt_m\mid R}(\xh_m,\xt_m;r)=\prod_{j\in m}P_{X_j}(x_j)P_{X_j}(\xt_j)
\]

where $m=\{j:r_j=1\}$ and $o=\{1,\dots,p\}\setminus m$. Therefore, from Lemma \ref{lem:factor}, $\Xh_m,\Xt_m$ are \pe conditioned on $R=r$.

Next, we show the conditional joint distribution of observed variables remains intact under MCAR.

\begin{subequations}\label{eq:uni_o}
\begin{align}
        P_{\Xt_o,\Xh_o\mid R}(\xt_o,\xh_o;r)&=P_{\Xt_o\mid \Xh_o, R}(\xt_o;\xh_o,r)P_{ \Xh_o\mid R}(\xh_o;r)\\
        &=P_{\Xt_o\mid X_o}(\xt_o;\xh_o)P_{ X_o\mid R}(\xh_o;r)\\
        &=P_{\Xt_o\mid X_o}(\xt_o;\xh_o)P_{ X_o}(\xh_o)\\
        &=P_{\Xt_o, X_o}(\xt_o,\xh_o)
\end{align}
\end{subequations}

\ref{eq:uni_o}b follows from sampling distribution $P_{\Xt_o\mid X_o}$ and $\Xh_o=X_o$. \ref{eq:uni_o}c uses the MCAR assumption. Because $ P_{\Xt_o,\Xh_o\mid R}(\xt_o,\xh_o;r)=P_{\Xt_o, X_o}(\xt_o,\xh_o)$ and $P_{\Xt_o\mid X_o}$ is \pe with respect to $P_{X_o}$ conditioned on $R=r$, $\Xh_o,\Xt_o$ are \pe.

We next use the two conditional \pety statements to show the unconditional \pety of $\hat{X}$ and $\Xt$. For any set $S\subseteq\{1,\dots,p\}$, 

\begin{subequations}\label{proof:uni}
\begin{align}
        &P_{\hat{X},\Xt}((\hat{x},\xt)_\swap)\\
        &=\sum_{r\in\{0,1\}^p} P_{\hat{X},\Xt\mid R}((\hat{x},\xt)_\swap;r)P_{R}(r)\\
        &=\sum_{r\in\{0,1\}^p} P_{\Xh_m,\Xt_m\mid R}((\xh_m,\xt_m)_{\text{swap}(S\cap m)};r) P_{\Xt_o,\Xh_o\mid R}((\xt_o,\xh_o)_{\text{swap}(S\cap o)};r)P_{R}(r)\\
        &=\sum_{r\in\{0,1\}^p} P_{\Xh_m,\Xt_m\mid R}(\xh_m,\xt_m;r) P_{\Xt_o,\Xh_o\mid R}(\xt_o,\xh_o;r)P_{R}(r)\\
        &=\sum_{r\in\{0,1\}^p} P_{\hat{X},\Xt\mid R}(\hat{x},\xt;r)P_{R}(r)\\
        &=P_{\hat{X},\Xt}(\hat{x},\xt)
        % &=P_{X_o,X_m}(x_o,\hat{x}_m)
\end{align}
\end{subequations}

\ref{proof:uni}b uses the law of total probability, \ref{proof:uni}c follows from univariate sampling i.e. $\Xh_m,\Xt_m\indep \Xh_o, \Xt_o \mid R=r$. \ref{proof:uni}d follows from conditioned on $R=r$, $\Xh_m,\Xt_m$  are \pe and $\Xh_o,\Xt_o$ are \pe.

% $\hat{X}\sim P_{X}$ following Lemma \ref{lem:main1}

% \[(\hat{X},\Xt)_\swap \eqd \hat{X},\Xt\]

\end{proof}
\subsection{Proposition \ref{thm:err}}\label{app:err}

\begin{proof}[Proof of Proposition \ref{thm:err}]

The MSE of the univariate sampling $Y'$ is given as 

\begin{subequations}\label{eq:mse_uni}
\begin{align}
        \E[(Y-Y')^2]&=\E[Y^2]+\E[Y'^2]-2\E[Y]\E[Y']\\
        &=2\E[Y^2]-2\E[Y]^2\\
        &=2\var(Y)
\end{align}
\end{subequations}
The first line uses $Y\indep Y'$ and expectation is a linear operator. The second line follows from $Y\eqd Y'$.

The conditional MSE of the posterior sampled estimator $Y''$ is given by:

\begin{subequations}\label{proof:mse1}
\begin{align}
    \E[(Y-Y'')^2\mid X]&=\E[Y^2\mid X]+\E[Y''^2\mid X]-2\E[Y\mid X]\E[Y''\mid X]\\
    &=2\E[Y^2\mid X]-2\E[Y\mid X]^2\\
    &=2\var(Y\mid X)\\
\end{align}
\end{subequations}
The first line uses $Y\indep Y''\mid X$ and expectation is a linear operator. The second line uses $Y\eqd Y''$. Then, the MSE of $Y''$ is given as:
\begin{subequations}
\begin{align}
    \E[(Y-Y'')^2]&=\E[\E[(Y-Y'')^2\mid X]]\\
    &=2\E[\var(Y\mid X)]\\
    &=2(\var(Y)-\var(\E[Y\mid X]))\\
\end{align}
\end{subequations}

The first line uses law of iterated expectations and the last line uses the law of total variance.

From Eq. \ref{eq:mse_uni} and Eq. \ref{proof:mse1} it follows that $\E[(Y-Y'')^2]\leq\E[(Y-Y')^2]$. Because ${Y'''=\E[Y\mid X]}$ is the optimal MSE estimator \cite{bertsekas2008introduction}, it has the lowest MSE i.e. ${\E[(Y-Y''')^2]\leq \E[(Y-Y'')^2]}$. 
\end{proof}
\subsection{Proof of Theorem \ref{thm:latent}}\label{app:latent}

\begin{proof}[Proof of Theorem \ref{thm:latent}]

The theorem assumes when the joint distribution of the observations and posterior sample $P_{X,\Zh}$ equals to $P_{X,Z}$, sampling procedure results in \pe $X, \Xt$. Therefore, it's sufficient to show the joint distribution of the imputed observation vector and the posterior sample maintains the distribution $P_{X,Z}$. Formally, we need to show ${P_{\Xh,\Zh}(\xh, \zh)=P_{X,Z}(\xh, \zh)}$ holds. 

We first start with ${\zh \in \mathcal{Z}}$, $ {\xh\in \mathcal{X}}$ s.t. $P_{X_o,Z}(\xh_o,\zh)>0$ where $\mathcal{Z}$ and $\mathcal{X}$ are the domains of $P_{Z}$ and $P_{X}$ (respt.). Let ${\mathcal{R}\defeq \{r\in \{0,1\}^p:P_{X_o,R}(\xh_o,r)>0\}}$

\begin{subequations}\label{proof:theo_3}
\begin{align}
        P_{\Xh,\Zh}(\xh, \zh)&=\sum_{r\in \{0,1\}^p} P_{\Xh,\Zh\mid R}(\xh, \zh;r)P_{R}(r)\\
        &=\sum_{r\in \{0,1\}^p} P_{\Xh_m\mid\Zh,R}(\xh_m; \zh,r)P_{\Zh \mid \Xh_o, R}(\zh ; \xh_o, r)P_{\Xh_o \mid R}(\xh_o; r)P_{R}(r)\\
        &=\sum_{r\in \{0,1\}^p} P_{X_m\mid Z}(\xh_m; \zh)P_{Z \mid X_o}(\zh ; \xh_o)P_{X_o \mid R}(\xh_o; r)P_{R}(r)\\
        %check zero division?
        &=\sum_{r\in \{0,1\}^p} P_{X_m\mid Z, X_o}(\xh_m; \zh,\xh_o)P_{Z \mid X_o}(\zh ; \xh_o)P_{X_o \mid R}(\xh_o; r)P_{R}(r)\\
        &=\sum_{r\in \{0,1\}^p} P_{X_m, Z\mid X_o}(\xh_m, \zh;\xh_o)P_{X_o \mid R}(\xh_o; r)P_{R}(r)\\
        &=\sum_{r\in \{0,1\}^p} P_{Z\mid X_m, X_o}( \zh;\xh_m,\xh_o)P_{X_m\mid X_o}(\xh_m;\xh_o)P_{X_o \mid R}(\xh_o; r)P_{R}(r)\\
        &=\sum_{\forall r \in \mathcal{R}} P_{Z\mid X}( \zh;\xh)P_{X_m\mid X_o}(\xh_m;\xh_o)P_{X_o \mid R}(\xh_o; r)P_{R}(r)\\
        &=\sum_{\forall r \in \mathcal{R}} P_{Z\mid X}( \zh;\xh)P_{X_m\mid X_o,R}(\xh_m;\xh_o,r)P_{X_o \mid R}(\xh_o; r)P_{R}(r)\\
        &=P_{Z\mid X}( \zh;\xh) \sum_{\forall r \in \mathcal{R}} P_{X_m, X_o\mid R}(\xh_m,\xh_o; r)P_{R}(r)\\
        &=P_{Z\mid X}( \zh;\xh) \sum_{\forall r \in \mathcal{R}} P_{X\mid R}(\xh; r)P_{R}(r)\\
        &=P_{Z\mid X}( \zh;\xh) P_{X}(\xh)\\
        &=P_{X,Z}(\xh,\zh)
        % P_{\hat{Z}_t\mid \hat{Z}_{t+1},X_{o(t)}}(z_t;z_{t+1},x_{o(t)})
\end{align}
\end{subequations}
\ref{proof:theo_3}a uses the total law of probability. \ref{proof:theo_3}b uses the chain rule and conditional independence resulting from the order the random vectors are sampled. \ref{proof:theo_3}c uses both $\Xh_o=X_o$ and the conditional distributions used to sample $\Xh_m$ and $\Zh$. \ref{proof:theo_3}d uses $X_m \indep X_o \mid Z$ and $P_{X_o\mid Z}(\xh_o;\zh)>0$. \ref{proof:theo_3}e follows from chain rule. \ref{proof:theo_3}f uses chain rule. \ref{proof:theo_3}g uses $\{1,\dots,p\}=m\cup o$, and for all $r\notin \mathcal{R}$ the inner summation terms are equal to zero i.e. $P_{X_o\mid R}(\xh_o;r)=0$. \ref{proof:theo_3}h uses MAR (or MCAR) assumption i.e. $X_m\indep R \mid X_o $ and $P_{X_o,R}(\xh_o,r)>0$. Using the equality $P_{X_m\mid X_o}=P_{X_m\mid X_o, R}$ was inspired by the Example 2 of Section 3.1.1.  \cite{mohanGraphicalModelsInference2017}. \ref{proof:theo_3}i uses distributive property and chain rule. \ref{proof:theo_3}j again uses $\{1,\dots,p\}=m\cup o$. \ref{proof:theo_3}k follows from the total low of probability and for all $r\notin \mathcal{R}$, $P_{X,R}(\xh,r)=0$. \ref{proof:theo_3}l uses the definition of conditional probability.

We now turn our attention to the remaining variables ${\zh \in \mathcal{Z}}$, $ {\xh\in \mathcal{X}}$ s.t.  $P_{X_o,Z}(\xh_o,\zh)=0$. Then, $P_{X,Z}(\xh,\zh)=0$ and $P_{Z\mid X_o}(\zh;\xh_o)=0$ also holds. From \ref{proof:theo_3}c 

\begin{equation*}
    \begin{split}
        P_{\Xh,\Zh}(\xh, \zh)&=\sum_{r\in \{0,1\}^p} P_{X_m\mid Z}(\xh_m; \zh)P_{Z \mid X_o}(\zh ; \xh_o)P_{X_o \mid R}(\xh_o; r)P_{R}(r)\\
        &=0\\
        &=P_{X,Z}(\xh,\zh)
    \end{split}
\end{equation*}
\end{proof}
% P_{\Xh,\Zh}(\xh, \zh)
% \input{tex/proof_sesia}
% \input{tex/proof_gz}
% \clearpage
\subsection{HMM Latent Variable Posterior Sampling}
\begin{prop}\label{thm:hmm_post}
Let $\hat{Z}$ denote the output of Algorithm \ref{alg:hmm_post} with the input $X_o$, then the resulting latent posterior distribution satisfies $P_{\hat{Z}\mid X_o}(z;x_o)=P_{Z\mid X_o}(z;x_o)$.
\end{prop}

To show that Algorithm \ref{alg:hmm_post} provides valid posterior samples we first prove to two useful lemmas. Our proof is an extension of the proof of Proposition 3 in \cite{sesiaGeneHuntingHidden2019} to the setting with missing values. We denote $o\cap\{1,\dots,t\}$ as $o(t)$.

\begin{lem}\label{lem:post_hmm}

If $\alpha_t(z_t)$ is calculated as in Algorithm \ref{alg:hmm_post} then,
$\alpha_t(z_t)=P_{Z_t,X_{o(t)}}(z_t,x_{o(t)})$.
\end{lem}
\begin{proof}

Proof by induction:

Base:
% P_{Z_t,X_{o(t)}}(z_t,x_{o(t)})
\begin{subequations}\label{eq:lem_3_1}
\begin{align}
  \alpha_1(z_1)&=\begin{cases}
    P_{X_1\mid Z_1}(x_1;z_1)P_{Z_1}(z_1),&\text{if } 1\in o\\
    P_{Z_1}(z_1),  &\text{o.w.}
\end{cases}\\&=
\begin{cases}
    P_{Z_1,X_1}(z_1,x_1),&\text{if } 1\in o\\
    P_{Z_1}(z_1),  &\text{o.w.}
\end{cases}\\
&=P_{Z_t,X_{o(1)}}(z_1,x_{o(1)})
\end{align}
\end{subequations}

\ref{eq:lem_3_1}a follows from Algorithm \ref{alg:hmm_post}. \ref{eq:lem_3_1}b uses the definition of conditional indepedence. \ref{eq:lem_3_1}c uses the definition of $x_{o(1)}$.

Induction step k:

\begin{subequations}\label{eq:lem_3_2}
\begin{align}
\gamma_{k}(z_k)&\defeq \sum_{z_{k-1}}P_{Z_k\mid Z_{k-1}}(z_k; z_{k-1})\alpha_{k-1}(z_{k-1})\\
&=\sum_{z_{k-1}}P_{Z_k\mid Z_{k-1}}(z_k; z_{k-1})P_{Z_{k-1},X_{o(k-1)}}(z_{k-1},x_{o(k-1)})\\
&=\sum_{z_{k-1}}P_{Z_k\mid Z_{k-1},X_{o(k-1)}}(z_k; z_{k-1},x_{o(k-1)})P_{Z_{k-1},X_{o(k-1)}}(z_{k-1},x_{o(k-1)})\\
&=\sum_{z_{k-1}}P_{Z_k, Z_{k-1},X_{o(k-1)}}(z_k, z_{k-1},x_{o(k-1)})\\
&=P_{Z_k,X_{o(k-1)}}(z_k,x_{o(k-1)})
\end{align}
\end{subequations}

\ref{eq:lem_3_2}b follows from the induction assumption at step $k-1$. \ref{eq:lem_3_2}c uses the conditional independence of the HMM. \ref{eq:lem_3_2}d uses the definition of conditional independence. \ref{eq:lem_3_2}e uses the law of total probability.

If $k\in o$, then 
\begin{subequations}\label{eq:lem_3_3}
\begin{align}
\alpha_k(z_k)&=P_{X_k\mid Z_k}(x_k;z_k)\gamma_{k}(z_k)\\
&=P_{X_k\mid Z_k,X_{o(k-1)}}(x_k;z_k,x_{o(k-1)})\gamma_{k}(z_k)\\
&=P_{X_k\mid Z_k,X_{o(k-1)}}(x_k;z_k,x_{o(k-1)})P_{Z_k,X_{o(k-1)}}(z_k,x_{o(k-1)})\\
&=P_{X_k, Z_k,X_{o(k-1)}}(x_k,z_k,x_{o(k-1)})\\
&=P_{Z_k,X_{o(k)}}(z_k,x_{o(k)})
% &=P_{Z_k,X_{o(k-1)}}(z_k,x_{o(k-1)})\\
% &=P_{Z_k,X_{o(k)}}(z_k,x_{o(k)})
\end{align}
\end{subequations}

\ref{eq:lem_3_3}a follows from Algorithm \ref{alg:hmm_post}. \ref{eq:lem_3_3}b follows from the conditional independence of HMM. \ref{eq:lem_3_3}c follows from Eq. \ref{eq:lem_3_2}. \ref{eq:lem_3_3}d follows from definition of conditional probability.

If $k\not\in o$, then 
\begin{subequations}\label{eq:lem_3_4}
\begin{align}
\alpha_k(z_k)&=\gamma_{k}(z_k)\\
&=P_{Z_k,X_{o(k-1)}}(z_k,x_{o(k-1)})\\
&=P_{Z_k,X_{o(k)}}(z_k,x_{o(k)})
\end{align}
\end{subequations}

\ref{eq:lem_3_4}a follows from Algorithm \ref{alg:hmm_post} as $k\not \in o$. \ref{eq:lem_3_4}b follows from Eq. \ref{eq:lem_3_2}. \ref{eq:lem_3_4}c follows from definition of $o(k)$.

\end{proof}

\begin{lem}\label{lem:post_hmm2}
% If $\alpha_t(z_t)$ is calculated as in Algorithm \ref{alg:hmm_post} then,
Let $P_{\hat{Z}_T\mid X_o}$ and $P_{\hat{Z}_t\mid \hat{Z}_{t+1},X_{o(t)}}$ denote the probabilities computed in Algorithm \ref{alg:hmm_post} then
${P_{\hat{Z}_t\mid \hat{Z}_{t+1},X_{o(t)}}(z_t; z_{t+1},x_{o(t)})=P_{Z_t\mid Z_{t+1},X_{o(t)}}(z_t; z_{t+1},x_{o(t)})}$ and ${P_{\hat{Z}_T\mid X_o}(z_T; x_o)=P_{Z_T\mid X_o}(z_T; x_o)}$
% \[P_{Z_t\mid Z_{t+1},X_{o(t)}}(z_t;z_{t+1},x_{o(t)})=\dfrac{P_{Z_{t+1}\mid Z_t}(z_{t+1};z_t)\alpha_{t}(z_t)}{\sum_{z_t'}P_{Z_{t+1}\mid Z_t}(z_{t+1};z_t')\alpha_{t}(z_t')}\]
\end{lem}
\begin{proof}

\begin{subequations}
\begin{align}
        P_{Z_t\mid Z_{t+1},X_{o(t)}}(z_t;z_{t+1},x_{o(t)})&=\dfrac{P_{Z_t,Z_{t+1},X_{o(t)}}(z_t,z_{t+1},x_{o(t)})}{P_{Z_{t+1},X_{o(t)}}(z_{t+1},x_{o(t)})}\\
        &=\dfrac{P_{Z_{t+1}\mid Z_t}(z_{t+1};z_t)\alpha_{t}(z_t)}{\sum_{z_t'}P_{Z_{t+1}\mid Z_t}(z_{t+1};z_t')\alpha_{t}(z_t')}\\
        &=P_{\hat{Z}_t\mid \hat{Z}_{t+1},X_{o(t)}}(z_t;z_{t+1},x_{o(t)})
\end{align}
\end{subequations}
The first line follows from the definition of conditional probability. The second line uses chain rule, conditional independence of the HMM and $\alpha_{t}(z_t)=P_{Z_t,X_{o(t)}}(z_t,x_{o(t)})$ from Lemma \ref{lem:post_hmm}. The last equality follows from Algorithm \ref{alg:hmm_post}. Similarly, at $t=T$
\begin{subequations}
\begin{align}
        P_{Z_T\mid X_o}(z_T;x_o)&= \dfrac{P_{Z_T,X_o}(z_T,x_o)}{P_{X_o}(x_o)}\\
        &=\dfrac{\alpha_T(z_T)}{\sum_{z_T'}\alpha_T(z_T')}\\
        &=P_{\hat{Z}_T\mid X_o}(z_T;x_o)
\end{align}
\end{subequations}

The first line follows from definition of conditional probability. The second line from Lemma \ref{lem:post_hmm}. The third line follows from Algorithm \ref{alg:hmm_post}.
\end{proof}
% To proove the above statement we prove Lemmas

% let $\alpha_t(z_t)\defeq P_{Z_t,X_{o(t)}}(z_t,x_{o(t)})$. Assume $t\in o$, then
\begin{proof}[Proof of Proposition \ref{thm:hmm_post}]

The resulting $P_{\hat{Z}\mid X_o}$ from Algorithm \ref{alg:hmm_post} can be factored using the sampling structure as follows:

\begin{subequations}\label{eq:prop_2}
\begin{align}
        P_{\hat{Z}\mid X_o}(\hat{z};x_o)
        &=P_{\hat{Z}_T\mid X_o}(\hat{z}_T;x_o)\prod_{t=1}^{T-1}P_{\hat{Z_t}\mid \hat{Z}_{t+1:T},X_o}(\hat{z_t};  \hat{z}_{t+1:T}, x_o)\\
        &=P_{\hat{Z}_T\mid X_o}(\hat{z}_T;x_o)\prod_{t=1}^{T-1}P_{\hat{Z_t}\mid \hat{Z}_{t+1}, X_{o(t)}}(\hat{z_t}; \hat{z}_{t+1}, x_{o(t)})\\
        &=P_{Z_T\mid X_o}(\hat{z}_T;x_o)\prod_{t=1}^{T-1} P_{Z_t\mid Z_{t+1},X_{o(t)}}(\zh_t; \zh_{t+1},x_{o(t)})\\
        &=P_{Z_T\mid X_o}(\zh_T;x_o)\prod_{t=1}^{T-1} P_{Z_t\mid Z_{t+1:T},X_o}(\zh_t;\zh_{t+1:T},x_o)\\
        &=P_{Z\mid X_o}(\hat{z};x_o)
\end{align}
\end{subequations}

\ref{eq:prop_2}a uses the chain rule. \ref{eq:prop_2}b uses the conditional independence following from the sampling order. \ref{eq:prop_2}c follows from Lemma \ref{lem:post_hmm2}. \ref{eq:prop_2}d follows from applying d-separation to the HMM graph. \ref{eq:prop_2}e again uses the chain rule. 
\end{proof}

\section{}
\section{Knockoffs Setup:}\label{app:knock}
In the model-x knockoffs framework one has to specify the feature-scorer and the final weighted score of each variable. As the feature-scorer we have used the coefficients of an L1 regularized logistic regression of the concatenated matrix $[\Xb,\Xtb]$ which optimizes the following objective function:

\[\hat{\beta}, \hat{\beta}_0 = \argmin_{\beta,\beta_0} \sum_{i=1}^N \log(1+e^{-y_i(\beta^T[x^{(i)},\xt^{(i)}]+\beta_0)})+\lambda \norm{\beta}_{1}\]

In each trial $\lambda$ is selected using 5-fold-cross-validation with area under the curve metric and search space $\{1e-10,1e-2,1e-1,1,1e1\}$ is used. Scikit-learn library \cite{scikit-learn} is used for the implementation. Let $\lambda_{cv}$ denote the resulting parameter and $\hat{\beta}(\lambda_{cv})\in \real^{2p}$ denote the estimated coefficients, the feature scores and the final scores are given by: $i=1,\dots, p$, $T_i=|\hat{\beta}(\lambda_{cv})_i|$ and $\Tt_i=|\hat{\beta}(\lambda_{cv})_{i+p}|$. 
\section{HMM Experiments}
\subsection{HMM Simulation Parameters}\label{app:hmm}

We have used the simulation parameters in \cite{sesiaGeneHuntingHidden2019}. Let $Z_t$ denote the t'th hidden states and $X_t$ the t'th explonatory variable both are categorical R.Vs with range \{0,\dots,8\}. The transmission and emission probabilities given as follows: 

\[P_{Z_1}(x)=\begin{cases}
    1,&\text{if } x=1\\
    0,              &\text{otherwise}
\end{cases}\]
\[
P_{Z_t\mid Z_{t-1}}(x;y)=\begin{cases}
    0.9,&\text{if } x=y,\\
    0.1,&\text{if } x=y+1 \\
    0.1,&\text{if } x=0, \ y= 8\\
    0,              &\text{otherwise}
\end{cases}
\]
\[
\]
\[P_{X_t\mid Z_{t}}(x;z)=\begin{cases}
    0.35/2,&\text{if } x=z\\
    0.35/2,&\text{if } x=z+1 \\
    0.35/2,&\text{if } x=0, z=8\\
    0.65/7, &\text{otherwise}
\end{cases}
\]

\subsection{Additional Results}

We included the power and FDR figures for our modified Sesia HMM Knockoffs (Algorithm \ref{alg:sesia}). We have also provided constant power contour plots of both posterior sampling + Sesia HMM and modified Sesia HMM Knockoffs in Fig. \ref{fig:contour}.

\begin{figure}[!htb]
    \centering
    \includegraphics[width=1.\linewidth]{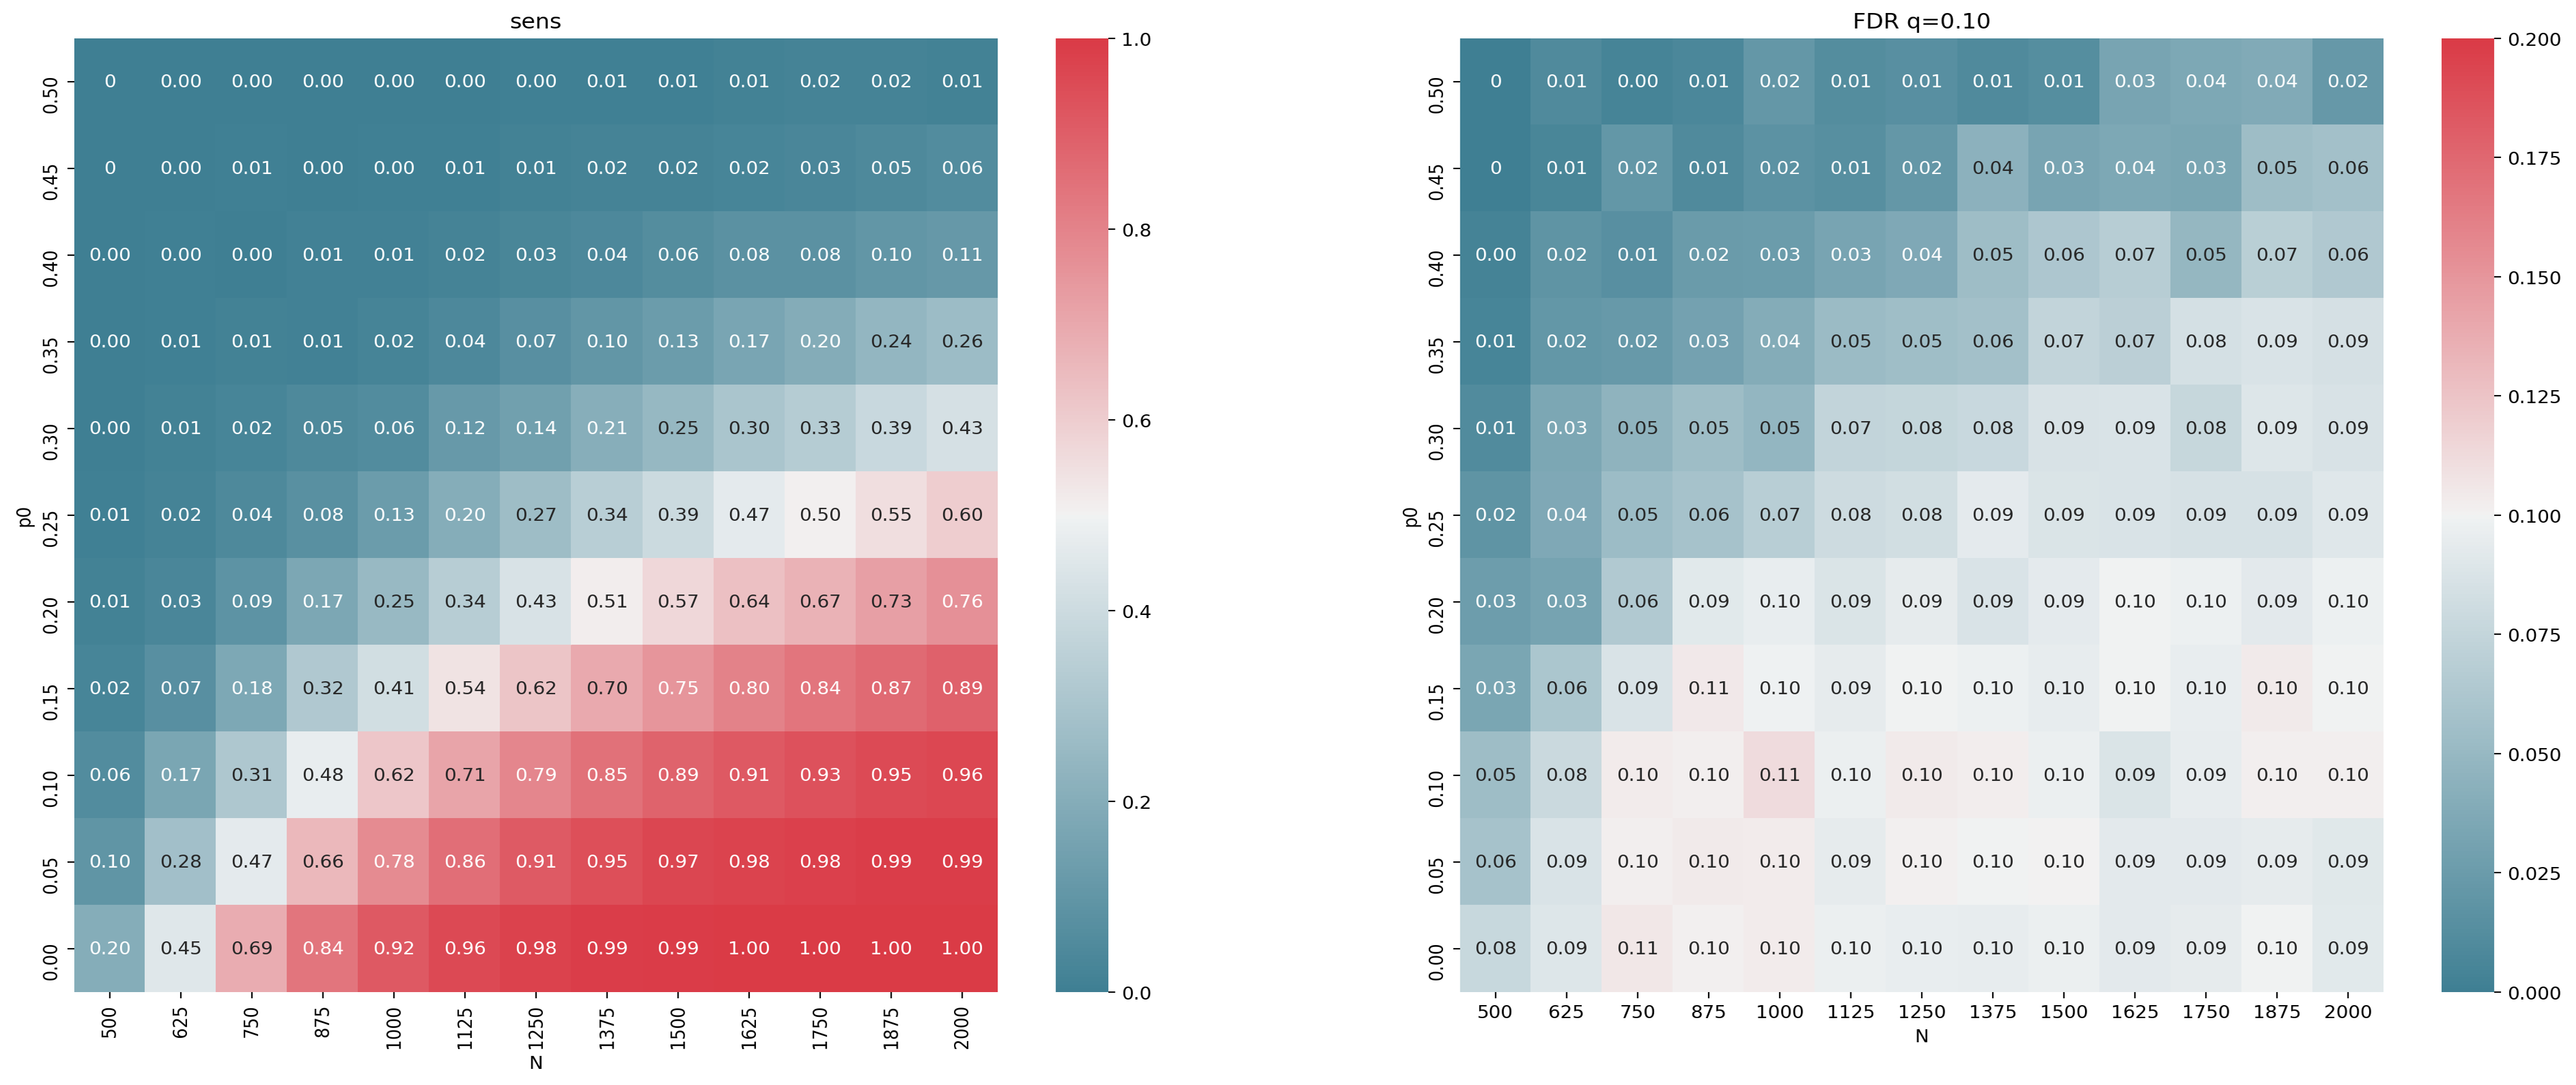}
    % {img/Picture2_fill.png}
    \caption{Heatmap of power on the left, FDR on right. Modified Sesia HMM Knockoffs (Algorithm \ref{alg:sesia}) is used. On the left darker red (blue) indicates higher (lower) power. On the right values above $q=0.1$ are red and below are blue.}
    \label{fig:heatmap2}
\end{figure}

\begin{figure}[!h]
    \centering
    \includegraphics[width=1.\linewidth]{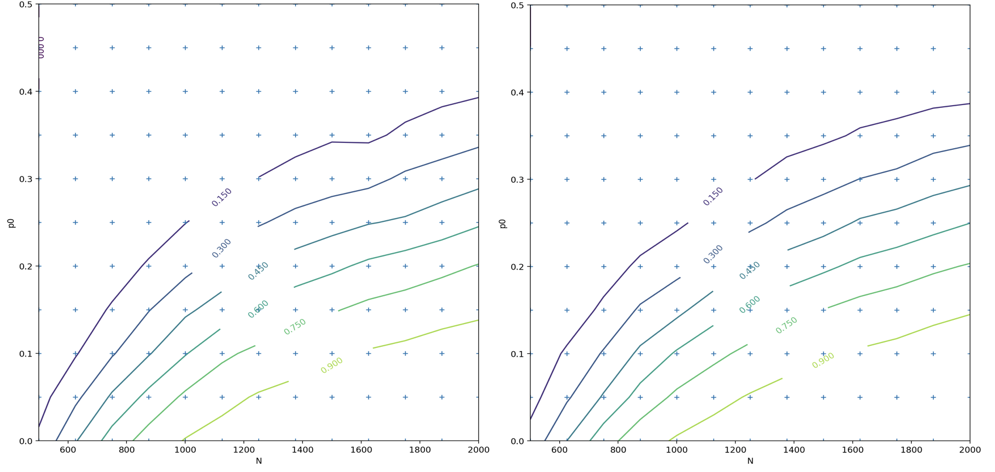}
    \caption{Contour plots of power. Each cross is a searched pair. Interpolation is used to to draw constant power lines. Left: the posterior imputation + Sesia HMM Knockoffs (Algorithm \ref{alg:main}), Right is the Modified Sesia HMM Knockoffs (Algorithm \ref{alg:sesia})}
    \label{fig:contour}
\end{figure}
